# Supplementary material for: Thermoelectric Scanning Gate Interferometry on a Quantum Point Contact
Source: arXiv:1804.00075 source file (2019-03-15)
Supplement: Supplementary file 1 [file Brun_supplemental.pdf]

# Thermoelectric Scanning Gate Interferometry on a Quantum Point Contact - Supplemental materials -

B. Brun[1], F. Martins[1], S. Faniel[1], A. Cavanna[4], C. Ulysse[4], A.Ouerghi[4], U. Gennser[4], D. Mailly[4], P. Simon[5], S. Huant[2], M. Sanquer[3], H. Sellier[2], V. Bayot[1] & B. Hackens[1]
[1]*IMCN/NAPS, Université catholique de Louvain, B-1348 Louvain-la-Neuve, Belgium*
[2]*Université Grenoble Alpes, CNRS, Institut Néel, 38000 Grenoble, France*
[3]*Université Grenoble Alpes, CEA, INAC-Pheliqs, 38000 Grenoble, France*
[4]*Centre de Nanosciences et Nanotechnologies (C2N) CNRS, Route de Nozay, F-91460 Marcoussis, France*
[5]*Laboratoire de Physique des Solides, Bâtiment 510, Université Paris Sud, F-91405 Orsay, France*

## I. SUBBANDS ENERGY SPACING

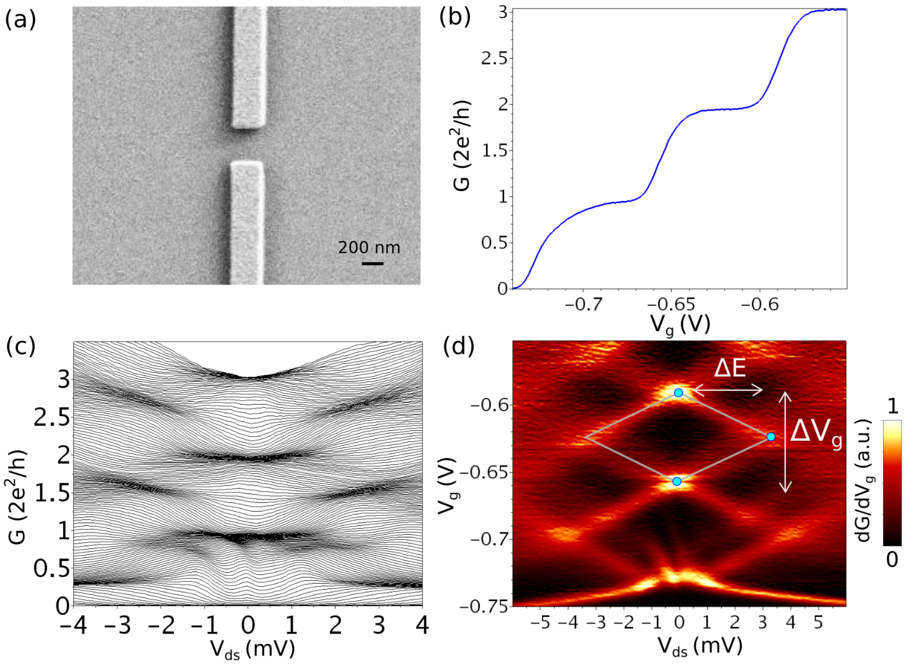


FIG. S1: **Lever-arm parameter of the split gate**: (a) Electron microscope image of device, and scheme of the heating current. (b) Differential conductance $G$ versus gate voltage $V_g$ , measured in 4-probes at 25 mK. (c) Non-linear conductance traces $G(V_{ds})$ for gate voltages spaced by 1.25 mV. (d) Derivative of $G$ versus $V_g$ as a function of $V_{ds}$ and $V_g$, showing the energy spacing $\Delta E$ between the quasi-1D subbands, which are separated by $\Delta V_g$ in gate voltage.

The lever-arm parameter $\alpha$ of the split gate, relating the potential energy in the constriction to the voltage applied on the split gate, is deduced from the non-linear conductance traces shown in Fig. S1 (c) and (d). The energy spacing between the first and second subband is $\Delta E_{1-2} = 3.5$ meV, and corresponds to a change in gate voltage $\Delta V_g = 0.065$ V. The lever-arm parameter of the split gate is therefore taken as $54 \pm 5$ meV/V.

## II. ZERO-BIAS CONDUCTANCE ANOMALY

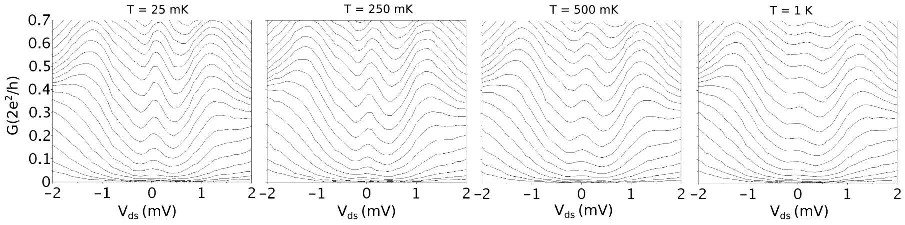


FIG. S2: **Evolution of the zero-bias anomaly with temperature:** Non-linear conductance traces $G(V_{ds})$ for gate voltages spaced by 1.25 mV versus DC source-drain bias $V_{ds}$, at 25 mK, 250 mK, 500 mK and 1 K.

The zero-bias anomaly is visible below the first conductance plateau. At a base temperature of 25 mK its full-width at half maximum is $\Delta V \sim 300$ $\mu$eV. This corresponds to a Kondo temperature $T_K = \frac{e\Delta V}{k_B} \sim 1.7$ K. The ZBA shades off for temperatures above 500 mK and has almost disappeared at 1 K.

## III. BACKGROUND IN THE THERMOELECTRIC SIGNAL

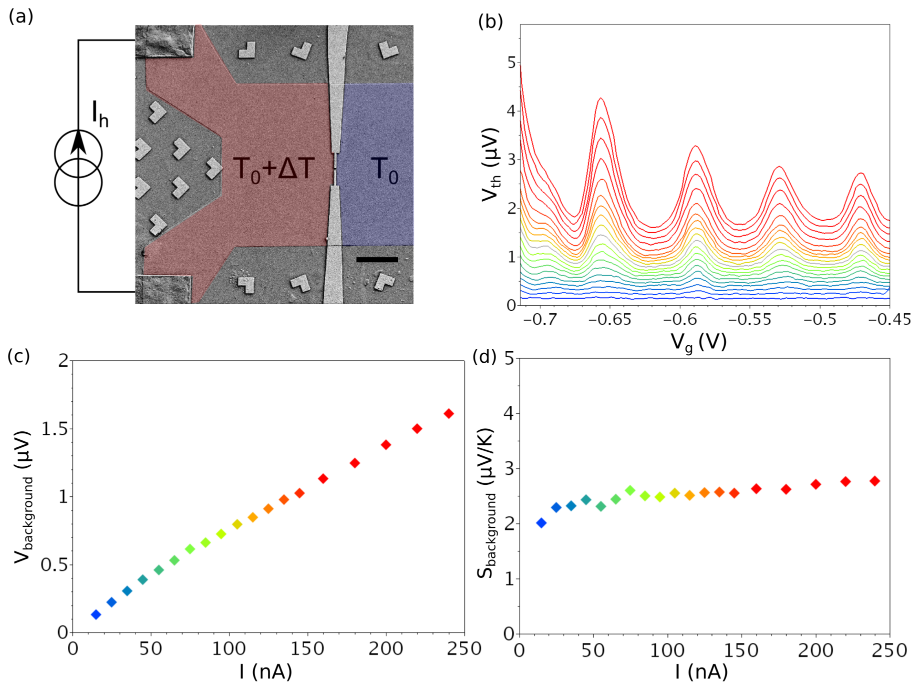


FIG. S3: **Temperature-dependent background in the thermoelectric voltage:** (a) Electron microscope image of the device. The scale bar is 5 $\mu$m. (b) Raw data of the measured $V_{th}$ versus $V_g$, for heating currents ranging from 15 nA (blue curve) to 240 nA (red curve). (c) Minimum thermovoltage between the first and second thermovoltage peaks at $V_g = -0.62$ V, plotted as a function of the heating current. This value corresponds to the gate-voltage-independent background which is subtracted in Fig. 2a of the main paper before the evaluation of the temperature difference. (d) Seebeck coefficient of the background signal obtained by dividing the thermovoltage by the estimated temperature difference $\Delta T$, extracted using the Mott's law (Fig. 2b of the main paper)

In our experimental setup, the thermoelectric voltage is measured between two ohmic contacts and includes several contributions : (i) the thermovoltage across the QPC which is the interesting signal, (ii) a thermovoltage in the 2DEG due to a temperature gradient inside the heated reservoir, and (iii) a thermovoltage at the junction between the heated 2DEG reservoir and the ohmic contact. We assume here that the ohmic contacts are thermalized at the fridge temperature. The thermovoltage at the QPC is the gate-voltage-dependent signal, whereas the two others contributions form the gate-voltage-independent signal, called background (see Fig. S3a). longbibliography For each heating current, the background is defined as the thermovoltage value in the second minimum of the curve, at $V_g = -0.62$ V. Since the temperature of both reservoirs is always kept lower than the subband energy spacing ($\Delta E/k_B \sim 40$ K), we indeed have $dG/dV_g = 0$ on the plateaus, and the thermovoltage at the QPC should drop to zero. The dependence of this background on the heating current is shown in Fig. S3b. Using the evaluated temperature differences as a function of the heating current (see main paper), we can estimate the thermopower corresponding to the observed background (Fig.S3c), and we find a value around 2.5 $\mu$V/K which depends weakly on the heating current.

In the following, we discuss quantitatively the origin of this background signal. The thermopower of the 2DEG can be separated in two main contributions: the thermopower due to the phonons, usually called the phonon drag, and the diffusion thermopower, that can be expressed as:

$$S^d = \frac{\pi^2 k_B^2 T}{3eE_F}(p+1) \tag{1}$$

where p represents the dependence of the electrons scattering rate with energy, that depends on the scattering mechanism but is close to unity [1]. In our case, this expression yields $S^d = 0.1$ $\mu$V/K at the lowest temperature, and rises up to $S^d = 0.5$ $\mu$V/K for the largest applied temperature differences. The 2DEG diffusion thermopower can therefore not account alone for this background. The contribution of phonons could be invoked, but it is likely that

the phonon drag does not contribute to the thermopower in our case, due to the sub-Kelvin temperature, regarding other works[1–3]. The thermopower due to the ohmic contacts is not well characterized, and might be responsible for this background signal, together with a small contribution from the 2DEG as discussed above.

## IV. TEMPERATURE ESTIMATED FROM SHUBNIKOV-DE-HAAS (SDH) OSCILLATIONS

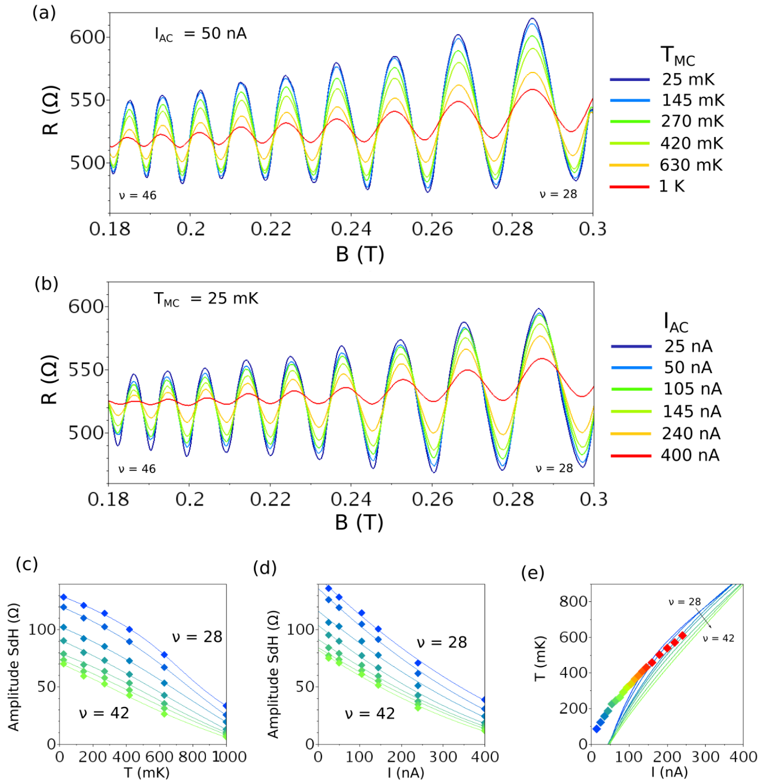


FIG. S4: **Temperature and AC current dependence of Shubnikov-de-Haas oscillations:** (a) SdH oscillations for temperatures ranging from 25 mK to 1 K. The applied AC current is 50 nA and a series resistance of 2.4 kΩ is subtracted to account for filters and contacts resistance (2-probes measurements). (b) SdH oscillations for AC current ranging from 25 nA to 400 nA at the base temperature of 25 mK. (c) Amplitude of SdH oscillations as a function of mixing chamber temperature, and polynomial fit for each Landau level. (d) Amplitude of SdH oscillations as a function of applied AC current, and polynomial fit for each Landau level. (e) Combination of the two polynomial fits to obtain temperature as a function of AC current. The temperature of the hot reservoir extracted from the thermovoltage analysis using the Mott's law is plotted as squares for comparison.

To reproduce the same geometry as in the thermopower measurement, the SdH oscillations (Fig. S4a and S4b) are measured between the two contacts located on the same side of the QPC, and a split gate voltage lower than the depletion threshold is applied. We used $V_g$ = -0.65 V corresponding to one mode open in the QPC but we checked that the results do not change if the QPC is closed at $V_g$ = -0.75 V. Fig. S4e presents the estimation of the current-induced 2DEG temperature obtained from the analysis of the SdH oscillations amplitude versus temperature (Fig. S4c) and versus current (Fig. S4d). The estimated temperatures vary a bit with the filling factor, but remain in the same range. This estimation indicates a similar order of magnitude as the temperatures evaluated from the thermovoltage analysis using the Mott's law (squares). The similarities between the two methods disappear below 300 mK. This is not surprising as the temperature evolution of the SdH oscillations was measured with a large current of 50 nA to have a reliable signal, corresponding to a current-induced temperature of about 200 mK.

It shall also be noted that the temperature profile is expected to be non-uniform in the heated region [4]. Hence SdH oscillations may be affected by the overall temperature profile whereas the estimated temperature difference obtained from the QPC thermovoltage is sensitive to the local temperature in its close vicinity. This could account for the observed differences between the two methods.

The sub-linear dependence of the temperature difference on heating current (Fig. S4e here and Fig. 2b of the main paper) can be explained in the framework of heat dissipation in 2DEGs. When electrons are brought to an electronic

temperature $T_e$ higher than the phonon temperature $T_{ph}$ they can lose energy via different mechanisms. The dominant ones at low temperatures are the phonon emission [5], which evolves as $T_e^5$, and the electron out-diffusion in the ohmic contacts, which evolves as $T_e^2$ as accurately verified down to the quantum limit of a single electronic channel [6, 7]. These competing losses yield a non-uniform temperature profile and a sub-linear dependence of the local temperature on the heating current [4].

## V. CORRELATION BETWEEN PHASE SHIFT AND CHANGE IN THE NUMBER OF LOCALIZED CHARGES

In Fig.S5 we explain how the phase shifts of the interference fringes are connected with a change by one in the number of charges localized in the QPC. The QPC presented here has the same geometry as the one in the present paper but is a different sample. Its transport charlongbibliographyacteristic are detailed in ref.[8]. We describe here our understanding of this phenomenon, which is a generic feature and is not sample specific, and has also been reproduced since by an other group. (Beat Braem, ETH Zürich, *private communication*).

Below the first conductance plateau, the 1D electronic density in the QPC is so low that a definite number of charges spontaneously localize due to Coulomb repulsion, in a mechanism similar to Wigner crystallization. This number of charges can be changed by moving the tip in front of the QPC, which affects the QPC potential and the size of the crystal. This effect is visible as concentric rings in the SGM image recorded below the first plateau Fig.S5a. These rings correspond to alternating single-peak or split-peak zero-bias anomalies (Fig.S5d) matching respectively with an odd or even number of localized charges. Dashed lines on Fig.S5a indicate tip positions leading to a change in the number of localized charges.

The number of localized charges can also change as a function of QPC opening (with $V_g$, not shown here). The modulations visible in the conductance traces at zero bias are really generic and correspond to a ZBA that spontaneously splits as the QPC opens or its shape is varied [9–11]. The tip position and gate voltage affect differently the number of localized charges but *loci* of changes in this number can be followed in colormaps of conductance versus $V_g$ and $d_{tip}$, as indicated by dashed lines in Fig.S5g and S5h.

Along the scan line 1, the changes in the number of charges is the only phenomenon affecting transport, hence they are easy to follow. Along line 2 however, this is less trivial. The tip that depletes the 2DEG underneath is scanned above preferential electron trajectories (branching). As a consequence, Fabry-Pérot interference fringes as a function of tip position are visible. Nevertheless, changes in the number of charges can still be visualized by differentiating the signal with respect to $V_g$, and interference can be highlighted by differentiating the signal with respect to $d_{tip}$. By placing dashed lines corresponding to a change in the number of localized charges on Fig.S5j and S5k, one can see that a change in this number is correlated with an abrupt phase shift of $\pi$ in the interference fringes. The most visible case is highlighted in Fig.S5l. This case is clearer because the tip is far from the QPC, hence changes in the number of charges are spaced by more than 100 nm in the tip position. When the tip is closer to the QPC, the phase shift is really hard to distinguish because these changes are separated by less than one hundred nanometer, which corresponds to only one or two Fabry-Pérot oscillations. It is therefore very difficult to see a phase shift by $\pi$ occurring only for one or two interference fringes, which leads to blurred and very large oscillations.

For the sample whose data are discussed in the main text, we were forced to scan the tip close to the QPC due to a dust particle on the sample surface, located at about 1 $\mu$m away from the QPC. In this region, the number of localized charges changes rapidly with tip position and produce several phase shifts in the interference pattern. In Fig. 4c of the main paper, there are probably two changes in the number of localized charges that produce the two distortions visible in the interference pattern.

The abrupt phase shift observed in TSGM as a function of gate voltage at the very pinch-off (Fig. 4d of the main paper) looks really similar to those observed in SGM in previous samples, but it differs in two main aspects:
- It evolves parallel to the QPC pinch-off line controlled by the cross-talk between the split gate and the scanning gate, whereas other observed phase shifts follow a different evolution (the green dashed lines in Fig.S5 are not parallel the line corresponding to the cross-talk)
- It is visible at very low transmission, lower than for any phase shift observed by the authors in their previous works.
These two differences suggest that, in the regime of very low transmission, the localized charges are not sensitive to the tip potential, whose only effect is to curve the pinch-off line.

A more puzzling property of this phase shift is that it is only visible in the thermovoltage and not in the conductance. We currently have no explanation for this anomalous behavior. Even if we know that the Mott's law does not hold in this regime of strong electron interactions, one would not expect such an all-or-nothing difference (phase shift or no phase shift) between the thermopower and the conductance. This really surprising difference indicates indeed that the thermopower and the conductance are significantly different spectroscopic tools, and may be sensitive to different aspects of an interacting mesoscopic system.

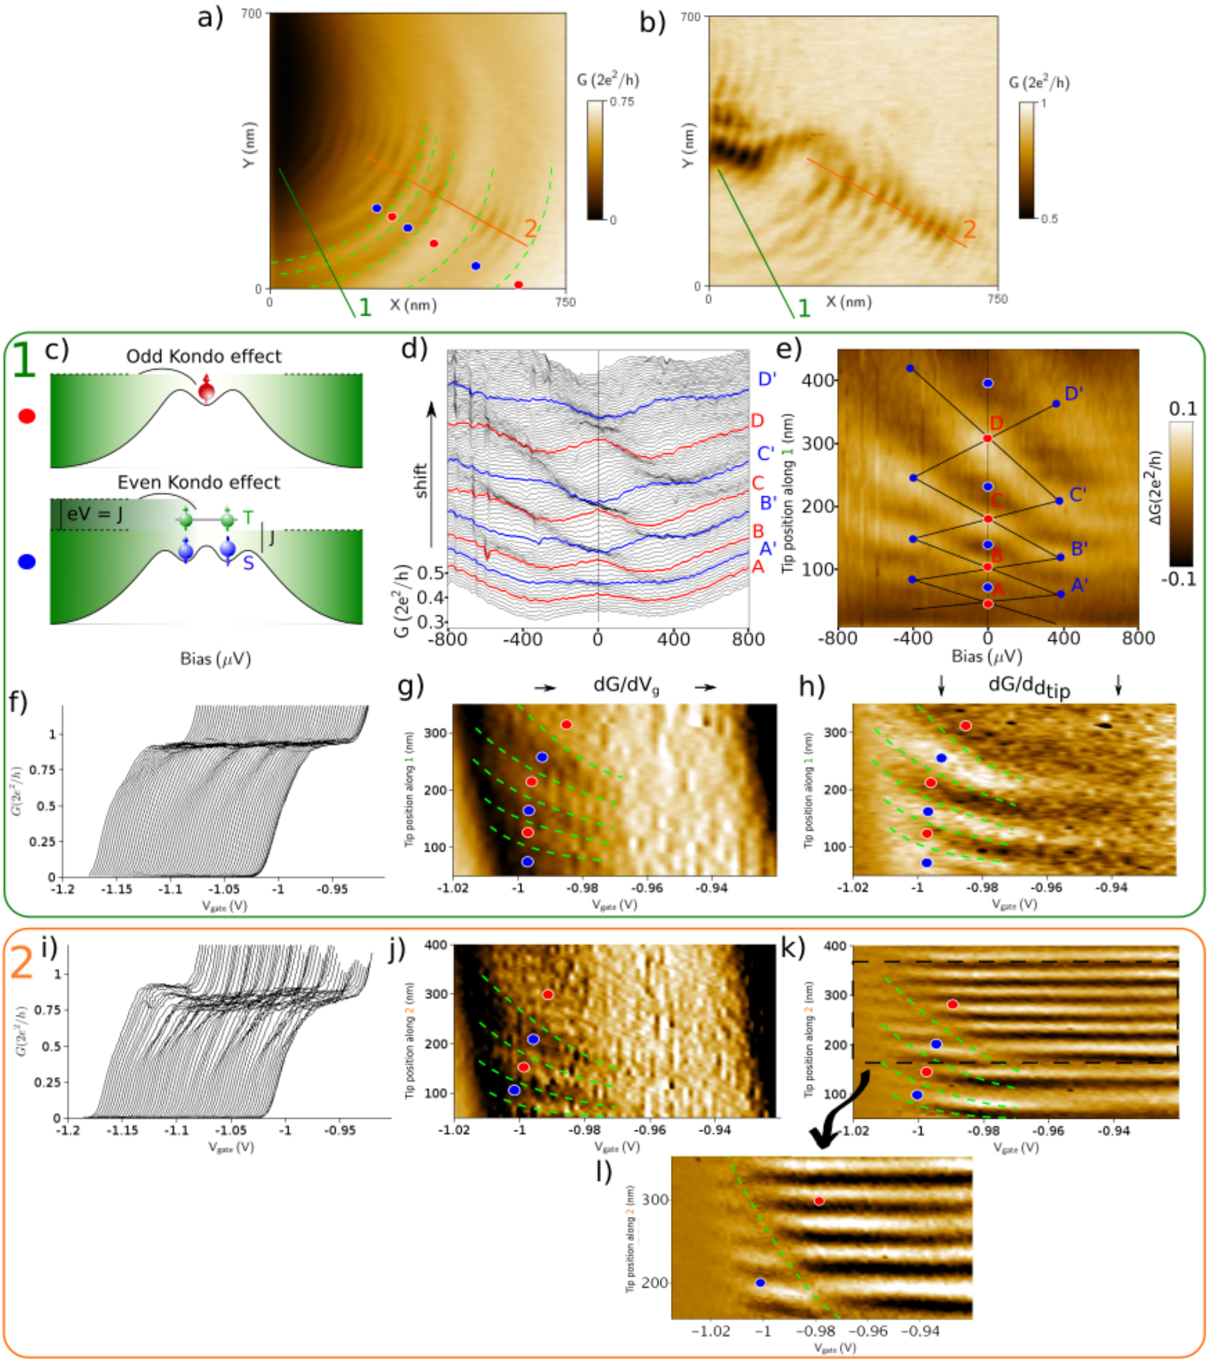


FIG. S5: **Correspondence between phase shifts in the interference fringes and changes in the number of localized charges, in a similar sample (see Ref. [8]):** (a,b) SGM maps of the conductance $G$ for gate voltages: (a) below the first plateau at $V_g = -1$ V and (b) on the first plateau at $V_g = -0.95$ V. (c) Scheme of spontaneously localized charges with a net spin S=1/2 ground state (upper panel) and a net spin S=0 ground state (lower panel). (d) Differential conductance $G$ versus source-drain bias at a fixed gate voltage $V_g$ = -1 V for different tip positions from 0 to 450 nm along the line 1 indicated in (a,b). Successive curves are shifted upwards by $0.0075 \times 2e^2/h$. (e) Color plot of the same data as in (d) after subtraction of a smooth background to suppress the main gating effect of the tip. Peak positions are indicated by dots. The successive ZBA splittings give a checkerboard pattern. (f,i) Traces $G(V_g)$ for several tip positions along the lines 1 and 2 indicated in (a,b). The curves are shifted in $V_g$ for clarity. (g,j) Color-plot of the same data, differentiated with respect to gate voltage ($\partial G/\partial V_g$). (h,k) Color-plot of the same data, differentiated with respect to tip position along these lines ($\partial G/\partial d_{tip}$). The different parities of the number of charges localized in the QPC are indicated by blue (even) and red (odd) dots. Green dashed lines represent changes by one electron charge. (l) Zoom of (k) showing a region with a single change in the charge number, highlighting a phase shift of the interference.

## VI. CLASSICAL ELECTROSTATIC SIMULATIONS

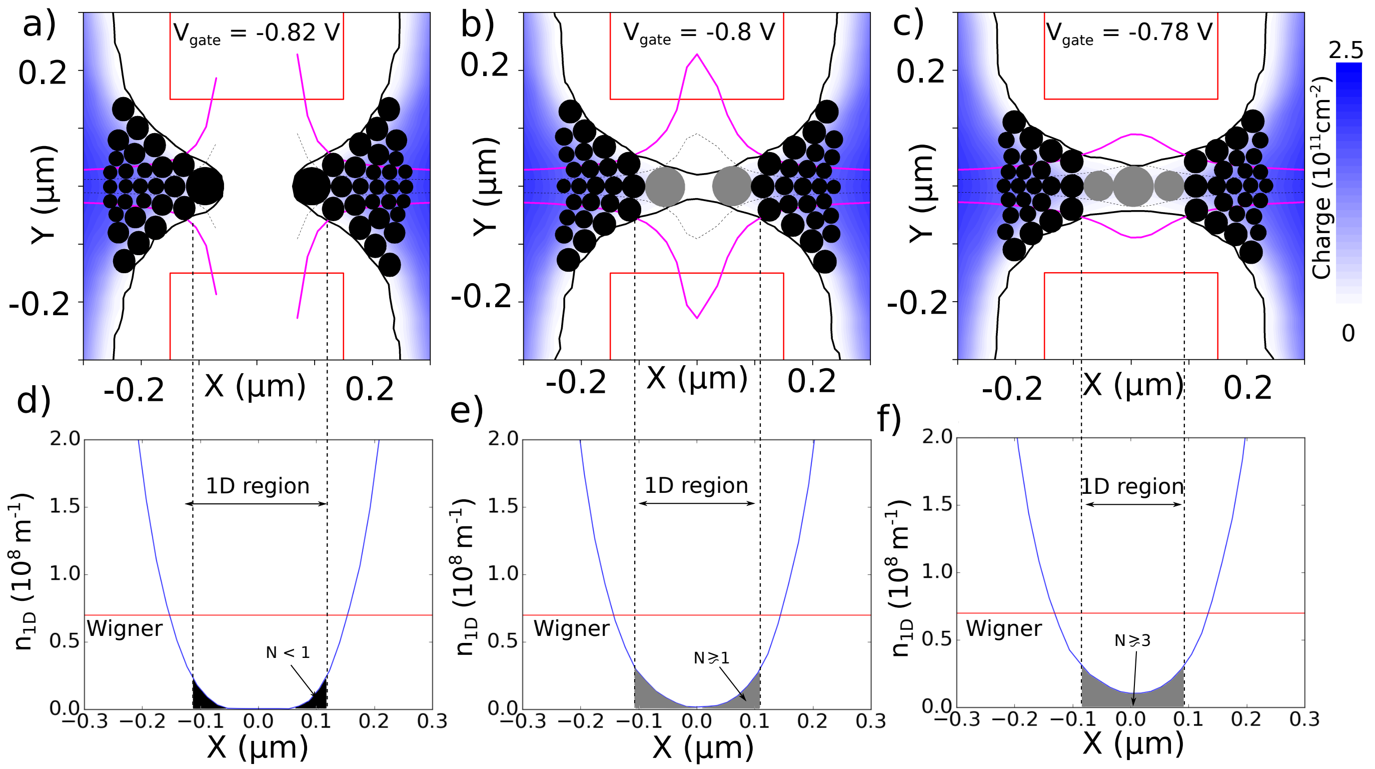


FIG. S6: Self-consistent electrostatic simulations for different gate voltages: (a) $V_{gate}$ = -0.82 V. (b) $V_{gate}$ = -0.8 V. (c) $V_{gate}$ = -0.78 V. The Fermi energy is $E_F$ = 8 meV. Red lines: gates geometry. Colorscale: 2D-density in the 2DEG plane. The spacing between the dashed lines indicate the electron spacing, and each black or grey disk contains one electron charge. The spacing between the two pink lines give the Fermi wavelength, and the 1D region corresponds to the region where these lines intersect with the zero-density black lines. The blue lines in (d-f) represent the 1D electron density integrated along the $y$-direction. In the 1D region (dashed lines), the 1D density is below the critical value for 1D Wigner crystallization.

We perform self-consistent classical electrostatic simulations to estimate how a localized state could form in our geometry, near pinch-off. The mesh grid is computed using Gmsh (http://gmsh.info) and the electrostatic problem is solved self-consistently using a modified version of MaxFEM (http://www.usc.es/en/proxectos/maxfem), an electromagnetic simulation software based on the finite element method.

The system is modeled by a 2DEG of density $2.5 \times 10^{11}$ cm$^{-2}$, separated by a 100 nm-thick AlGaAs layer from the surface, on top of which 300 nm-wide and 100 nm-thick metallic gates are defined. The local density is computed in the Thomas-Fermi approximation and represented as a colormap in Fig.S6a-c for different gate voltages. The surface occupied by each electrons is then represented by a circle whose diameter is equal to $\sqrt{1/n_{2D}}$.

To estimate how many electrons are likely to localize in the QPC channel, we compare these results with the expected criterion for Wigner crystallization. As the density of an electronic system is reduced, the Wigner-Seitz radius $r_s$, defined as the ratio of half the inter-particle distance to the Bohr radius $a_B$, enlarges ($a_B$ = 10 nm in GaAs). When $r_s$ overcomes the critical value $r_{sc}$, the electronic system undergoes a phase transition from a Fermi liquid to a Wigner crystal[12]. In two dimensions, numerical estimates of $r_{sc}^{2D}$ indicate a value close to 37[13], which is never reached in our simulations. The Fermi liquid description therefore holds for the 2D regions. In one dimension however, the value of $r_{sc}^{1D}$ depends on the confinement potential strength but is closer to unity [14]. In Ref.[8], $r_{sc}^{1D}$ has been estimated to $\sim 0.7$, and this criterion was shown to be reached below the first conductance plateau, yielding a few crystallized electrons in the channel. In Figs. S6d to S6f, we show estimates of the 1D density $n_{1D}$ in the one-dimensional region, and indicate the region where the electron transport is effectively 1D, i.e. where only one transverse electronic mode is permitted. In this 1D region, the 1D density is below the critical density $1/(2r_{sc}^{1D}a_B)$ where we can expect Wigner crystallization (below the red line). In the following, we calaculate how many electrons the crystallization region may contain. This estimation shows that no crystallization is expected for a completely closed QPC (Fig.S6a,d), since both 1D regions on the two sides of the QPC barrier contain less than one electron

charge. As the QPC opens, the density in the two 1D regions on both sides of the barrier increase, up to a point where each of these regions may contain one electron charge (Fig.S6b,e). For larger opening, the crystallization regions merge across the full QPC length and becomes large enough to contain 3 electrons (Fig.S6c,f).

Though a more accurate calculation including quantum effects would be required to estimate the exact behavior of localized electrons[15, 16], our simple approach indicates that one electron may be localized in each 1D region olongbibliographyf the channel near QPC pinch-off (Fig.S6b), but this situation is not favored anymore as the QPC closes (Fig.S6a). Therefore the energy level corresponding to this spontaneously localized state may evolve in a very peculiar way with the QPC opening, and could correspond to the behavior of the phase shift observed in our TSGM experiment.


[1] V. C. Karavolas and P. N. Butcher, *Diffusion thermopower of a 2DEG*, Journal of Physics: Condensed Matter **3**, 2597 (1991).

[2] R. Fletcher, P. T. Coleridge, and Y. Feng, *Oscillations in the diffusion thermopower of a two-dimensional electron gas*, Phys. Rev. B **52**, 2823–2830 (1995).

[3] M. Schmidt, G. Schneider, C. Heyn, A. Stemmann, and W. Hansen, *Thermopower of a 2D Electron Gas in Suspended AlGaAs/GaAs Heterostructures*, Journal of Electronic Materials **41**, 1286-1289 (2012).

[4] A. Mittal, R. Wheeler, M. Keller, D. Prober, and R. Sacks, *Electron-phonon scattering rates in GaAs/AlGaAs 2DEG samples below 0.5 K*, Surface Science **361**, 537 - 541 (1996).

[5] P. J. Price, *Hot electrons in a GaAs heterolayer at low temperature*, Journal of Applied Physics **53**, 6863-6866 (1982).

[6] S. Jezouin, F. D. Parmentier, A. Anthore, U. Gennser, A. Cavanna, Y. Jin, and F. Pierre, *Quantum Limit of Heat Flow Across a Single Electronic Channel*, Science **342**, 601–604 (2013).

[7] E. Sivre, A. Anthore, F. D. Parmentier, A. Cavanna, U. Gennser, A. Ouerghi, Y. Jin, and F. Pierre, *Heat Coulomb blockade of one ballistic channel*, Nat. Phys. **14**, 145 (2017).

[8] B. Brun, F. Martins, S. Faniel, B. Hackens, G. Bachelier, A. Cavanna, C. Ulysse, A. Ouerghi, U. Gennser, D. Mailly, S. Huant, V. Bayot, M. Sanquer, and H. Sellier, *Wigner and Kondo physics in quantum point contacts revealed by scanning gate microscopy*, Nat. Commun. **5**, 4290 (2014).

[9] S. M. Cronenwett, *Coherence, charging and spin effects in quantum dots and quantum point contacts*, Ph.D. thesis, Harvard University, 2001.

[10] M. J. Iqbal, *Electron many-body effects in quantum point contacts*, Ph.D. thesis, Groningen University, 2014.

[11] B. Brun, *Electron interactions in mesoscopic physics : Scanning Gate Microscopy and interferometry at a quantum point contact*, Ph.D. thesis, Université de Grenoble, October 2014.

[12] E. Wigner, *On the Interaction of Electrons in Metals*, Phys. Rev. **46**, 1002–1011 (1934).

[13] B. Tanatar and D. M. Ceperley, *Ground state of the two-dimensional electron gas*, Phys. Rev. B **39**, 5005–5016 (1989).

[14] L. Shulenburger, M. Casula, G. Senatore, and R. M. Martin, *Correlation effects in quasi-one-dimensional quantum wires*, Phys. Rev. B **78**, 165303 (2008).

[15] A. D. Güçlü, C. J. Umrigar, H. Jiang, and H. U. Baranger, *Localization in an inhomogeneous quantum wire*, Phys. Rev. B **80**, 201302 (2009).

[16] T. Rejec and Y. Meir, *Magnetic impurity formation in quantum point contacts*, Nature **442**, 900–903 (2006).
